# Supplementary material for: Coupling Physics Informed Neural Networks with External Solvers
Source: arXiv:2509.24615 source file (2025-09-29)
Supplement: Supplementary file 1 [file Appendix.tex]

\section{\bf{Appendix}}\label{sec:Appendix}
